# Supplementary material for: OmniVid: A Generative Framework for Universal Video Understanding
Source: arXiv:2403.17935 source file (2024-03-26)
Supplement: Supplementary file 1 [file X_suppl.tex]

\clearpage
%\setcounter{page}{1}
%\maketitlesupplementary

\section{Additional Experimental Results}
\subsection{Joint $v.s.$ Separate Training.} We jointly train \system across different video tasks with each distinguished by a specific task indicator, and compare the results with separate training in Figure~\ref{fig:joint}. Benefiting from a unified output space, joint training demonstrates the potential to enhance or, at least, sustain performance in classification and captioning tasks. However, we also observe noticeable performance degradations in localization tasks. We attribute this to the intricate nature of spatial-temporal localization tasks, which require diverse fine-grained modeling of video features, consequently, joint training introduces inherent challenges for model optimization.

\begin{figure}[!ht]
\centering
\includegraphics[width=\linewidth]{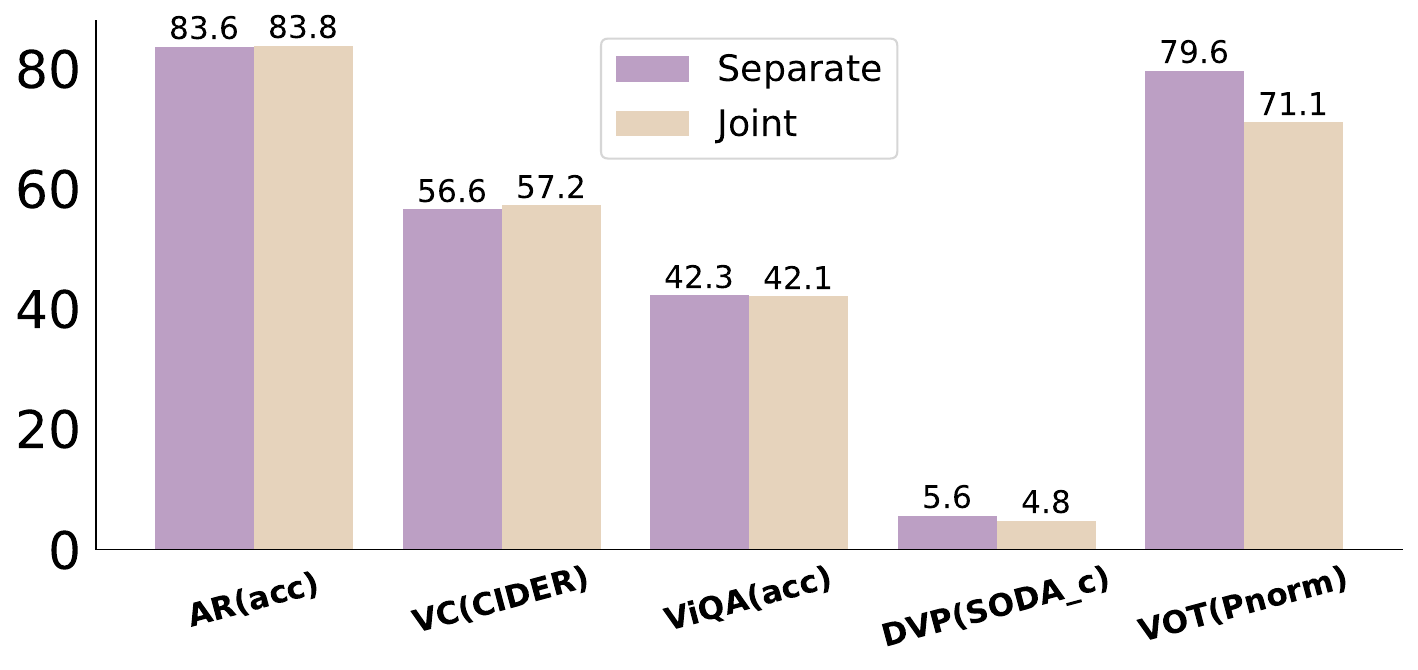}
\vspace{-0.3in}
\figcaption{Comparison between joint and separate training.}
\label{fig:joint}
\end{figure}

\subsection{Initialization of Video Encoder.}  We initialize the video encoder with different weights, including the model pre-trained on ImageNet21K~\cite{deng2009imagenet} and Kinetics-400~\cite{kay2017kinetics}. The results in Table~\ref{tab:video_enc} show that a stronger video encoder, \ie, the model pre-trained on larger scale data, typically leads to better performance on various video tasks. Specially, even if our video encoder is trained on image data only, the results are still competitive.
\begin{table}[!ht]
\small
\centering
\vspace{-0.1in}
\caption{Effects of video encoder pretraining on \system.}
\vspace{-0.1in}
\setlength{\tabcolsep}{7.2pt}

\begin{tabular*}{\linewidth}{lc|ccccc }
\toprule
\textbf{Model} && \textbf{AR} & \textbf{CC} & \textbf{ViQA} & \textbf{DVP} & \textbf{VOT} \\
\midrule
IN21K && 82.5 & 50.6 & 37.4 & 5.2 & 78.5 \\
K400 && 83.0 & 56.1 & 42.0 & 5.6 & 79.3 \\
\rowcolor{Gray}
K600 (Ours) && \textbf{83.6} & \textbf{56.6} & \textbf{42.3} & \textbf{5.6} & \textbf{79.6} \\
\bottomrule
\end{tabular*}
\vspace{-0.1in}
\label{tab:video_enc}
\end{table}

\subsection{Effects of Model Size.} 

We also conduct experiments to try different variants of the video encoder and token decoder to study the effects of model size on the performance. Since VideoSwin only released the Base model pre-trained on K600, we use ImageNet-1k pre-trained models for comparison. As for the token decoder, we adopt T5~\cite{chung2022scaling} since Bart only released Base and Large models. 

The results in Table~\ref{tab:model_size} show that the size of video encoder has a larger influence than that of token decoder. Specifically, even with T5Small, \system could achieve competitive results on action recognition and clip captioning (compared to T5Base, the CiDEr on MSRVTT only drops 0.2).

\begin{table}[!ht]
\small
\centering
\vspace{-0.1in}
\caption{Effects of model size on different video tasks.}
\vspace{-0.1in}

\setlength{\tabcolsep}{0.5pt} % let TeX compute the intercolumn space
\begin{tabular*}{\linewidth}{@{\extracolsep{\fill}}lcc | cc | c @{}}
\toprule
\textbf{Pretrain} & \textbf{Model} && \textbf{AR} &&  \textbf{CC} \\
\midrule
IN1k & Ours (SwinTiny-BartBase) && 79.4 && 49.1 \\
IN1k & Ours (SwinSmall-BartBase) && 80.9 && 50.5 \\
IN1k & Ours (SwinBase-BartBase) && 81.1 && 51.0 \\
\midrule
IN1k+K600 & Ours (SwinBase-T5Small) && 83.4 && 56.3 \\
IN1k+K600 & Ours (SwinBase-T5Base) && 83.9 && 56.5 \\
IN1k+K600 & Ours (SwinBase-T5Large) && 83.5 && 56.9 \\
\midrule
IN1k+K600 & Ours (SwinBase-BartBase) && 83.6 && 56.6 \\
\bottomrule
\end{tabular*}
\label{tab:model_size}
\vspace{-0.18in}
\end{table}

\section{Failure Cases}

We carefully check the failure cases of \system for dense video captioning and show two representitative examples below. As can be seen, our method may fail to distinguish the events occurring within the same scene, \eg, ```\textit{A rough river is shown with a person riding off in the distance}''' and ```\textit{The person is seen riding in a kayak closer to the camera}''' in the first case. The reason lies in that in order to support end-to-end training of the model, we sample video frames sparsely (160 frames in total), making it susceptible to overlooking subtle activity changes. We believe this issue could be resolved by leveraging more efficient video encoders and dense sampling strategy.

\begin{figure}[!ht]
\centering
\includegraphics[width=\linewidth]{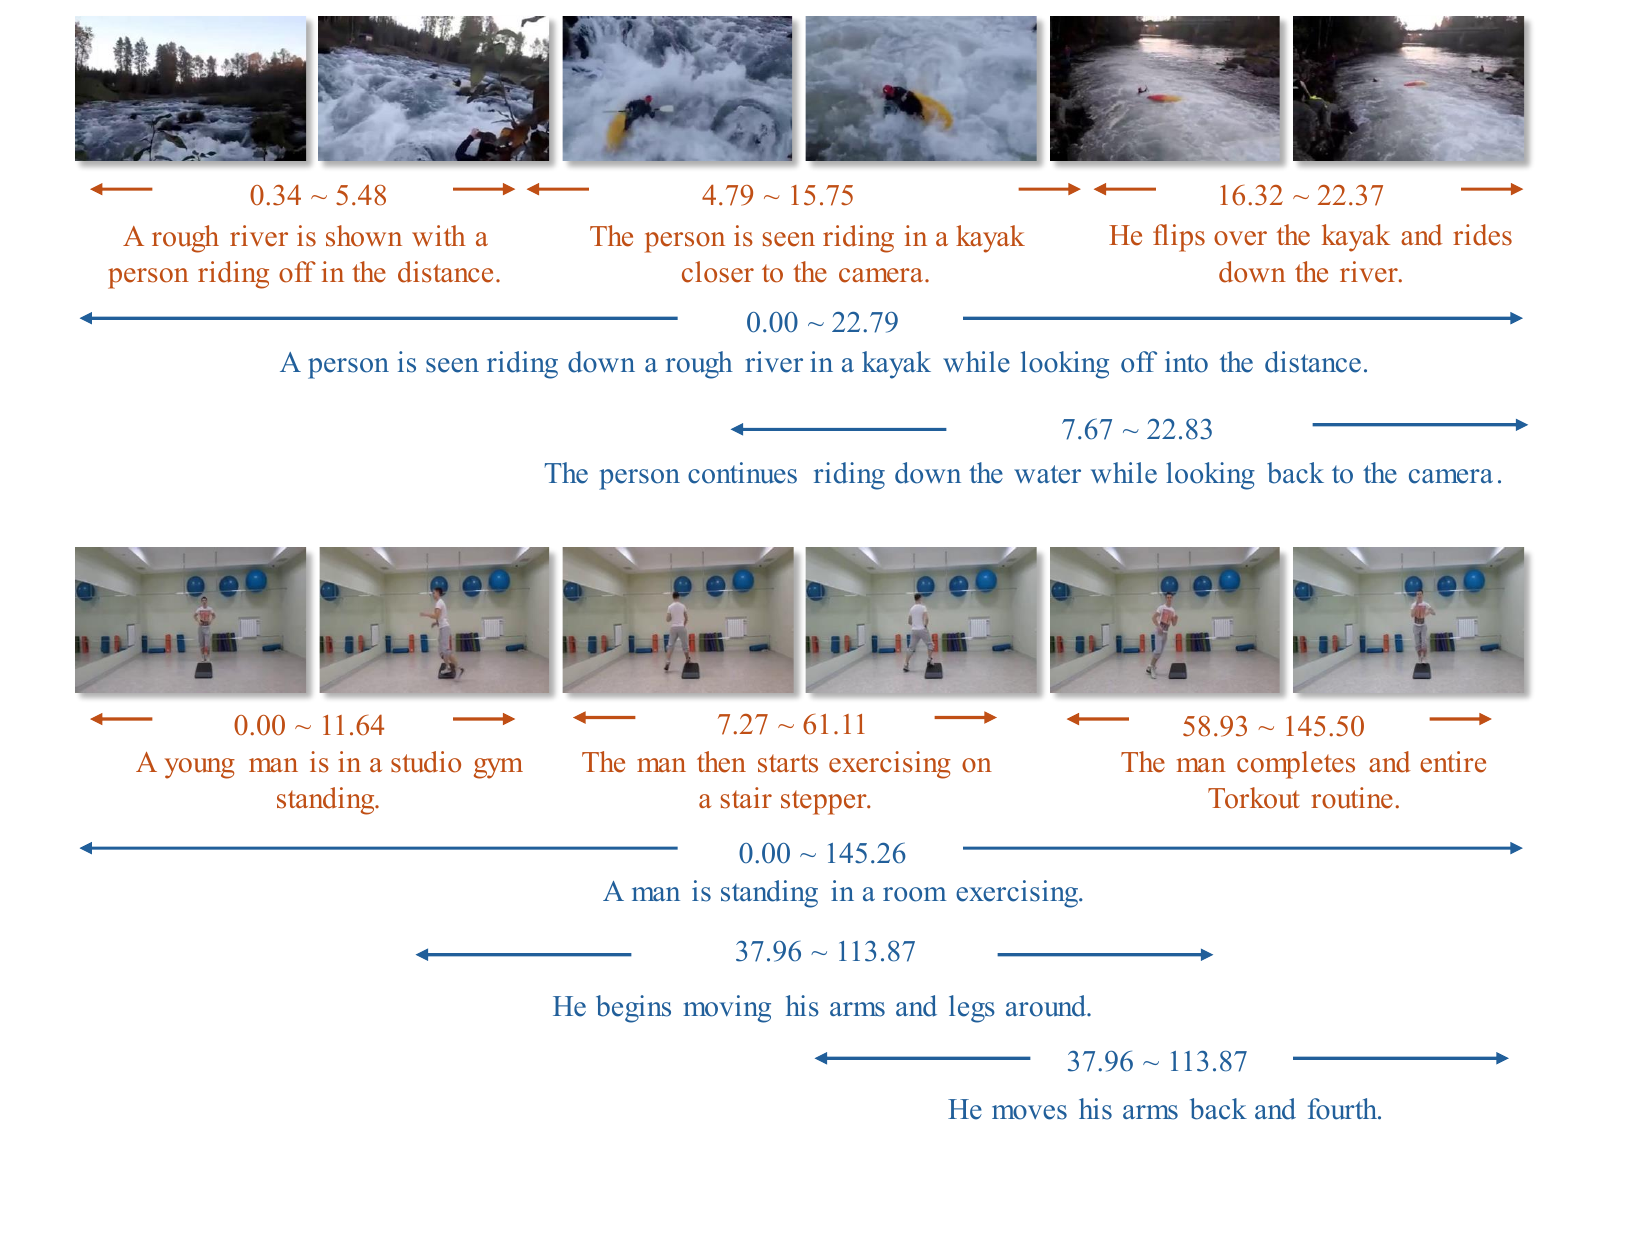}
\vspace{-0.25in}
\figcaption{Failure cases on ActivityNet for dense video captioning.}
\label{fig:anet}
\vspace{-0.1in}
\end{figure}
